# Supplementary material for: Capital Demand Driven Business Cycles: Mechanism and Effects
Source: arXiv:2110.00360 source file (2022-09-07)
Supplement: Supplementary file 1 [file appx_computation.tex]

In this section we provide details of the numerical approach used in the simulations of the Dynamic Solow model. The code was written in Python, utilising Cython for speedy implementations of the demand, and general case
